# Supplementary material for: HiP-AD: Hierarchical and Multi-Granularity Planning with Deformable Attention for Autonomous Driving in a Single Decoder
Source: arXiv:2503.08612 source file (2025-03-11)
Supplement: Supplementary file 5 [file supp_granularity.tex]

\begin{table}[tb]\footnotesize
\centering
\resizebox{0.75\linewidth}{!}
{
\begin{tabular}{l|c}
\toprule
Multi-granularity       & Sampling Strategy  \\        
\midrule
Temporal waypoints      & 2m, 5m   \\
Spatial waypoints       & 2Hz, 5Hz \\
Driving-style waypoints & 2Hz $\times$ 3, 5Hz $\times$ 3  \\
\bottomrule
\end{tabular}
}
\caption{The granularity of 10 used in our HiP-AD model, including the three types of driving-style waypoints, represents fast, medium, and slow speeds with high and low frequency.}
\label{tab:supp_granularity}
\end{table}
