# Supplementary material for: HiP-AD: Hierarchical and Multi-Granularity Planning with Deformable Attention for Autonomous Driving in a Single Decoder
Source: arXiv:2503.08612 source file (2025-03-11)
Supplement: Supplementary file 6 [file supp_num_modality.tex]

\begin{table}[tb]\footnotesize
\centering
\resizebox{0.8\linewidth}{!}
{
\begin{tabular}{c|cccc}
\toprule
\multirow{2}{*}{\textbf{Number}} & \multicolumn{4}{c}{\textbf{Closed-loop Metric}}  \\
& DS $\uparrow$  & SR(\%) $\uparrow$ & Eff. $\uparrow$ & Com. $\uparrow$\\ \midrule                           
18 & 86.56 & 62.27 & 197.21 & 17.35   \\
48 & \textbf{86.77} & \textbf{69.09} & \textbf{203.12} & \textbf{19.36}   \\
\bottomrule
\end{tabular}
}
\caption{Comparison of the number of modalities: `Eff.' and `Com.' are abbreviations for Efficiency and Comfort.}
\label{tab:supp_num_modality}
\end{table}
