# Supplementary material for: HiP-AD: Hierarchical and Multi-Granularity Planning with Deformable Attention for Autonomous Driving in a Single Decoder
Source: arXiv:2503.08612 source file (2025-03-11)
Supplement: Supplementary file 8 [file supp_sparse_global.tex]

\begin{table}[tb]\footnotesize
\centering
\resizebox{1\linewidth}{!}
{
\begin{tabular}{l|c|cc}

\toprule
\multirow{2}{*}{\textbf{Setting}}&\multirow{2}{*}{\textbf{Interaction}}&\multicolumn{2}{c}{\textbf{Closed-loop Metric}}\\
 &  & 
Driving Score$\uparrow$ &
Success Rate(\%)$\uparrow$ \\

\midrule
Global & Cross Attention & 73.4 & 49.1  \\
Sparse & Deformable Attention & \textbf{84.2} & \textbf{65.5} \\
\bottomrule
\end{tabular}
}
\caption{Comparison of Global and Sparse Interactions.}
\label{tab:supp_sparse_global}
\vspace{-0.5cm}
\end{table}
